# Supplementary material for: RA-RT: Robot Agents in Real Time via Learned Asynchronous Skill Scheduling
Source: arXiv:2611.40946 source file (2026-11-30)
Supplement: Supplementary file 1 [file X_suppl.tex]

\clearpage
\appendix
\section*{Supplementary Material}

\section{Training and Serving Details}
\label{sec:supp_training_serving}

Stage~1 fine-tunes the vision-frozen Qwen3.5-9B backbone for one epoch on the 55,412-sample SFT dataset ($64$K context length, global batch size $8$, $\text{lr}=10^{-5}$) across four RTX PRO 5000 GPUs, utilizing \texttt{ms-swift}~\cite{msswift}, DeepSpeed ZeRO-3~\cite{zero}, and sequence parallelism of 4 to manage memory constraints. Stage~2 trains rank-32 LoRA adapters on disjoint seeds via \cref{eq:post_loss} ($\text{lr}=8\times 10^{-6}$). Finally, Stage~3 merges the checkpoints, aligns the MTP drafting head (\cref{eq:mtp_kl}), and deploys the unified policy using \texttt{W8A16} quantization for low-latency serving on A800 and RTX PRO 5000 GPUs.

\section{Design Rationale, Negative Results, and Ablation Studies}
\label{sec:rationale}

Designing a compact embodied planner under a running wall-clock budget is fraught with counter-intuitive failure modes: optimizations that shorten per-turn latency can collapse multi-turn success rates, whereas post-training recipes or memory prompts that help long-horizon tasks can induce severe negative transfer on spatial disambiguation. Across more than 3,800 closed-loop evaluation episodes spanning sixteen full 145-position contract panels (\texttt{c2}--\texttt{c17}, plus three cross-hardware panels on 72\,GB NVIDIA RTX PRO 5000 Blackwell GPUs) and seventeen controlled 24-position development gates (\texttt{seed=2}, strictly disjoint from \texttt{seed=1} evaluation and \texttt{seeds 11--44} post-training rollouts), we systematically tested every architectural, runtime, memory, and post-training choice in \cref{sec:method}.

Below, we document both successful designs and negative attempts across six dimensions: (1) speculative decoding and serving inference (\cref{subsec:supp_serving}), (2) deliberation budget control (\cref{subsec:supp_thinking}), (3) prompt engineering and qualitative memory scoping (\cref{subsec:supp_memory}), (4) physical transition guardrails and concurrent tool dispatch (\cref{subsec:supp_guardrails}), (5) horizon-aware clean-scene restart budgeting (\cref{subsec:supp_restarts}), and (6) post-training paradigms including offline self-distillation, online RLOO, off-policy teacher distillation, and drift-free action-only weighting (\cref{subsec:supp_posttrain}). We then trace the end-to-end progression across full evaluation panels (\cref{subsec:supp_progression}) and report cross-backbone baseline comparisons powered by GPT-6.2-Sol (\cref{subsec:supp_frontier_baselines}).

\paragraph{Unified evaluation protocol.}
Unless noted otherwise, all full-panel numbers are measured under our unified contract (\texttt{seed=1}, $T_{\max}=1{,}800$\,s wall-clock budget, $N_{\max}=100$ turns, official thinking sampling $T=1.0, \text{top-}p=0.95, \text{top-}k=20, \text{presence\_penalty}=1.5$) over 148 task instances across LIBERO Standard (40 tasks), LIBERO-Pro object/task swaps (80 tasks), and LIBERO-Plus visual/language/camera perturbations (28 tasks). Development gates evaluate a stratified 24-position subset (8 Standard, 8 Pro, 8 Plus) on \texttt{seed=2}. Every episode records conservation-checked wall-clock components: planner prefill ($T_{\mathrm{prefill}}$, time-to-first-token), autoregressive decoding ($T_{\mathrm{dec}}$), real-time-paced 20\,Hz physics + RGB-D state capture ($T_{\mathrm{sim}}$), and VLA/SAM3 tool inference ($T_{\mathrm{perc/vla}}$). The main paper reports the unweighted mean of the three benchmark success rates, with denominators of 40, 80, and 28, respectively (\cref{tab:benchmark_results,tab:ablation_results}).

\begin{table}[t]
    \centering
    \caption{\textbf{Impact of aligned 6-step MTP speculative decoding (\texttt{c2}, \texttt{seed=1}).} Top: all completed contract episodes. Bottom: strictly paired 70-position subset. Distribution-matched MTP-6 doubles throughput ($2.01\times$) and increases task success by $+11.4$\,pp because fewer episodes time out mid-manipulation.}
    \label{tab:supp_mtp}
    \resizebox{\linewidth}{!}{
    \begin{tabular}{@{}lcccccc@{}}
        \toprule
        \textbf{Serving Variant} & \textbf{SR (\%)} & \textbf{Capped (s)} & \textbf{TTS (s)} & \textbf{Decode (tok/s)} & \textbf{Accept (tok/step)} & \textbf{$T_{\mathrm{dec}}$ (s)} \\
        \midrule
        w/o MTP (\texttt{c2:dec}, $n=71$) & 53.5 (38/71) & 1171.0 & 624.9 & 67.7 & 1.00 & 979.7 \\
        w/ MTP-6 (\texttt{c2:decopt}, $n=88$) & \textbf{63.6} (56/88) & \textbf{895.0} & \textbf{377.8} & \textbf{136.1} & \textbf{2.90} & \textbf{710.4} \\
        \midrule
        Paired w/o MTP ($n=70$) & 52.9 (37/70) & 1175.6 & 618.7 & 67.7 & 1.00 & --- \\
        Paired w/ MTP-6 ($n=70$) & \textbf{64.3} (45/70) & \textbf{905.7} & \textbf{408.8} & \textbf{136.1} & \textbf{2.90} & --- \\
        \bottomrule
    \end{tabular}
    }
\end{table}

\subsection{Speculative Decoding and Prefix-Preserving Serving}
\label{subsec:supp_serving}

Planner inference accounts for 80\%--95\% of active episode wall-clock time (\cref{eq:wall_conservation}), making autoregressive acceleration essential for closed-loop execution.

\paragraph{Aligned 6-step MTP decoding.}
Without speculative decoding, Qwen3.5-9B generates at 67.7\,tok/s and spends an average of 979.7\,s per episode in decoding alone (\cref{tab:supp_mtp}), causing nearly half of long-horizon episodes to exhaust the 1,800\,s budget mid-recovery. Adding our 6-step MTP head with vocabulary-subset projection and $(T,\text{top-}k,\text{top-}p)$-matched stochastic drafting raises mean acceptance to 2.90\,tok/step (136.1\,tok/s), and further draft-head alignment pushes acceptance to 3.28--3.36\,tok/step (158--165\,tok/s). On the strictly paired 70-task subset, this lossless $2.01\times$ speedup increases task success by $+11.4$\,pp ($52.9\% \to 64.3\%$) and reduces capped completion time by 269.9\,s.

\paragraph{Block-quantized KV compaction.}
Naive per-turn sliding-window truncation invalidates the KV cache on every turn once an episode exceeds 40 turns, pushing cumulative prefill time $T_{\mathrm{prefill}}$ above 180\,s. Quantizing the compaction boundary $c(L)$ to fixed 50-message blocks (\cref{eq:block_compaction}) alongside far-horizon image stabilization ($W_{\mathrm{img}}=8$) maintains a 74\%--90\% KV prefix-cache hit rate across 50--100-turn rollouts, keeping cumulative $T_{\mathrm{prefill}}$ within 55.5--63.4\,s per episode.

\paragraph{Unconstrained Phase-2 tool decoding.}
We also tested enforcing XGrammar structured JSON constraints during Phase~2 forced answers, which dropped validation success on the 24-task development split to 54.2\% (13/24), substantially below native unconstrained decoding. Hard logit masking distorts the model's post-deliberation token distribution and induces premature argument truncation; we therefore keep Phase~2 decoding unconstrained. 

\begin{table}[t]
    \centering
    \caption{\textbf{Ablation of deliberation modes and per-turn thinking budgets $B_{\mathrm{think}}$ on the 24-position development gate (\texttt{seed=2}).} Disabling or heuristically gating deliberation collapses spatial/perturbed success; unbounded thinking wastes wall-clock budget; $B_{\mathrm{think}}=2{,}048$ achieves the Pareto optimum.}
    \label{tab:supp_thinking}
    \resizebox{\linewidth}{!}{
    \begin{tabular}{@{}lccccccc@{}}
        \toprule
        \textbf{Deliberation Policy} & \textbf{SR (\%)} & \textbf{Std / Pro / Plus} & \textbf{Capped (s)} & \textbf{Active (s)} & \textbf{Turns} & \textbf{Out Tok} \\
        \midrule
        Heuristic gate, $B_{\mathrm{think}}=1024$ (\texttt{w1:gate\_b1024}) & 37.5 (9/24) & 2/8, 4/8, 3/8 & 1211.1 & 363.1 & 84.1 & 26.5K \\
        Thinking disabled (\texttt{w1:off}) & 45.8 (11/24) & 3/8, 3/8, 5/8 & 1042.8 & 304.1 & 76.4 & 21.1K \\
        Always on, $B_{\mathrm{think}}=1024$ (\texttt{w1:on\_b1024}) & 62.5 (15/24) & 5/8, 4/8, 6/8 & 778.9 & 365.2 & 57.5 & 33.8K \\
        Always on, unbounded (\texttt{w1:on\_base}) & 70.8 (17/24) & 6/8, 4/8, 7/8 & 919.5 & 956.5 & 53.0 & 105.0K \\
        \midrule
        Unbounded + hints (\texttt{w2:sys\_unb}) & 66.7 (16/24) & 4/8, 4/8, 8/8 & 912.4 & 912.8 & 36.4 & 105.7K \\
        Budget $B_{\mathrm{think}}=3072$ + hints (\texttt{w2:sys\_b3072}) & 79.2 (19/24) & 6/8, 5/8, 8/8 & 646.1 & 646.5 & 38.8 & 71.5K \\
        \textbf{Budget $B_{\mathrm{think}}=2048$ + hints (\texttt{w2:sys\_b2048})} & \textbf{87.5 (21/24)} & \textbf{8/8, 6/8, 7/8} & \textbf{606.0} & \textbf{591.7} & \textbf{39.7} & \textbf{62.0K} \\
        \bottomrule
    \end{tabular}
    }
\end{table}

\subsection{Deliberation Modes and Thinking-Budget Trade-offs}
\label{subsec:supp_thinking}

Under a shared wall-clock budget, explicit reasoning presents a direct trade-off: disabling deliberation speeds up individual turns but impairs spatial grounding and recovery, whereas unbounded reasoning consumes excessive inference time. We compare seven deliberation policies across two development waves on the 24-task \texttt{seed=2} validation split (\cref{tab:supp_thinking}). When a per-turn thinking budget $B_{\mathrm{think}}$ is enforced, generation stops at $B_{\mathrm{think}}$ reasoning tokens and appends a closing \texttt{</think>} tag on the cached KV state to trigger immediate tool-call generation.

Disabling chain-of-thought reasoning lowers per-turn token cost but causes spatial misgrounding and blind retries, increasing episode turns and dropping success from 70.8\% to 45.8\%. Triggering reasoning only after tool errors performs even worse (37.5\%), because physical failures---such as grasping a distractor bowl or stalling above a basket---still return nominal status codes and require geometric reasoning to diagnose. Conversely, unbounded reasoning averages over 105K output tokens per episode and spends excessive time deliberating on ambiguous frames, whereas capping too tightly ($B_{\mathrm{think}}=1{,}024$) truncates multi-object 3D coordinate comparisons mid-derivation (62.5\%). Setting $B_{\mathrm{think}}=2{,}048$ with concise tool-use hints resolves both failure modes: over 94\% of turns finish naturally within the budget, while longer deliberations transition directly to tool calls on the cached KV state. Compared to unbounded reasoning, this budget cuts output tokens by 41\%, saves over 300\,s per episode, and raises success from 66.7\% to 87.5\%. 

\begin{table}[t]
    \centering
    \caption{\textbf{Ablation of system-prompt hints and memory modes.} Overloading system prompts with dense physics rules (\texttt{d3w2}) or attaching memory globally onto easy object/spatial tasks (\texttt{d3w1:mem\_*}, \texttt{d4w1} Pro) causes file-reading distraction and degrades accuracy. Selective routing of denoised qualitative notes (\texttt{qualitative\_clean}) to long-horizon/goal tasks avoids distraction while recovering \texttt{pro/libero\_10\_task}.}
    \label{tab:supp_memory}
    \resizebox{\linewidth}{!}{
    \begin{tabular}{@{}llccc@{}}
        \toprule
        \textbf{Experiment / Setting} & \textbf{Memory \& Prompt Variant} & \textbf{Overall SR} & \textbf{Sub-benchmark Effect} & \textbf{Capped (s)} \\
        \midrule
        \texttt{d3w1} (\texttt{seed=2}, $n=24$) & Cold memory + workflow (\texttt{cold\_wf}) & \textbf{83.3\%} (20/24) & Pro: \textbf{7/8} & \textbf{573.7} \\
        \texttt{d3w1} (\texttt{seed=2}, $n=24$) & Global memory + workflow (\texttt{mem\_wf}) & 75.0\% (18/24) & Pro: 5/8 ($-2$) & 678.3 \\
        \texttt{d3w1} (\texttt{seed=2}, $n=24$) & Global memory + lite workflow (\texttt{mem\_wfl}) & 75.0\% (18/24) & Pro: 5/8 ($-2$) & 665.1 \\
        \texttt{d3w2} (\texttt{seed=2}, $n=24$) & Cold + dense physics prompt (\texttt{cold\_wf\_phy}) & 66.7\% (16/24) & All: 6/8, 5/8, 5/8 & 828.9 \\
        \midrule
        \texttt{c8} $\to$ \texttt{c9} (\texttt{seed=1}, $n=27$) & Unrouted short index on \texttt{std+plus libero\_10} & $44.4\% \to \mathbf{70.6\%}$ & $8/17 \to \mathbf{12/17}$ ($+4$) & $1177 \to \mathbf{910}$ \\
        \texttt{c8} $\to$ \texttt{c9} (\texttt{seed=1}, $n=9$) & Raw 16--45\,KB notes on \texttt{pro/10\_task} & $44.4\% \to 22.2\%$ & $4/9 \to 2/9$ ($-2$) & $1269 \to 1547$ \\
        \texttt{c9} $\to$ \texttt{c10} (\texttt{seed=1}, $n=9$) & Denoised $<4.7$\,KB notes (\texttt{qualitative\_clean}) & $22.2\% \to \mathbf{44.4\%}$ & $2/9 \to \mathbf{4/9}$ ($+2$) & $1547 \to \mathbf{1210}$ \\
        \bottomrule
    \end{tabular}
    }
\end{table}

\subsection{Prompt Engineering and Qualitative Memory Scoping}
\label{subsec:supp_memory}

We evaluate three strategies for injecting domain knowledge: global system-prompt rules, unrestricted task-memory access, and selectively routed qualitative notes (\cref{tab:supp_memory}).

\paragraph{System-prompt granularity.} Appending a 5-point embodied-mechanics checklist (covering post-release lateral retreats, grasp-before-contact ordering, handle-only grasps, swap-axis probing, and two-can wedging) to every episode reduces validation success from 83.3\% to 66.7\% and increases average duration from 573.7\,s to 828.9\,s. Execution traces show that on single-bowl and grocery-box tasks, the 9B planner over-applies lateral retreats and handle constraints, perturbing already-seated objects and wasting turns. Concise tool-schema shortcuts (\texttt{segment\_xyz} and \texttt{batch}) instead improve both speed and accuracy without side effects.

\paragraph{Task-selective memory routing.} Similarly, enabling task-memory retrieval across all suites drops LIBERO-Pro validation success from 87.5\% (7/8) to 62.5\% (5/8) and adds over 100\,s per episode. On straightforward single-goal tasks, exposing memory files distracts the planner into spending early turns querying notes via \texttt{read\_task\_memory} rather than relying on direct visual grounding.

\paragraph{Note denoising.}
Restricting qualitative notes to multi-step long-horizon tasks (\texttt{libero\_10}) avoids this distraction and lifts success across standard and visual-perturbation splits from 44.4\% to 70.6\% (cutting capped time from 1{,}177\,s to 910\,s), though raw notes initially reduce task-swapped long-horizon success from 44.4\% (4/9) to 22.2\% (2/9). Auditing these files reveals that unfiltered logs (16--45\,KB) contain dozens of archived failure trajectories that exceed our 10\,KB per-source excerpt limit, causing mid-sentence truncation and inducing the planner to imitate suboptimal recovery actions (e.g., partially closing a drawer before grasping). Stripping historical failure tables so every note fits under 4.7\,KB (\texttt{qualitative\_clean}) eliminates truncation, restores task-swapped long-horizon success to 44.4\% (4/9), and cuts average episode time by 337\,s (from 1{,}547\,s to 1{,}210\,s).

\subsection{Physical Transition Guardrails and Concurrency}
\label{subsec:supp_guardrails}

Through iterative ablation across full-benchmark evaluations, several seemingly reasonable low-level heuristics degraded performance before we converged on the final runtime guardrails in \cref{subsec:framework}:

\paragraph{Structured secondary masks vs.\ flat top-$k$ outputs.}
Returning flat top-$k$ segmentation masks confused the planner on LIBERO Standard ($32/40 \to 24/40$), whereas restricting outputs to the top-1 mask left duplicate-object swaps in LIBERO-Pro ambiguous. Formatting secondary detections under an explicit \texttt{alternate\_candidates} field with 2D bounding boxes and median \texttt{world\_xyz} coordinates resolved this ambiguity, restoring Standard to 32/40--34/40 (across evaluation runs) and helping lift Pro to 55/80 (68.8\%).

\paragraph{Empty-air gripper threshold ($0.0028$\,m vs.\ $0.0018$\,m).}
Lowering the \texttt{pi0\_pick} zero-load closure filter $\delta_{\mathrm{air}}$ from $0.0028$\,m to $0.0018$\,m to accommodate thin rims caused LIBERO-Plus success to drop from 24/28 to 18/28. Execution state traces showed that closed empty fingers under operational space control (OSC) compliance rest at $0.0020$--$0.0021$\,m, causing missed grasps to be misclassified as held objects. Restoring $\delta_{\mathrm{air}}=0.0028$\,m alongside coordinate-frame warnings on zoomed \texttt{selection\_crop} views immediately recovered LIBERO-Plus to 25/28 (89.3\%) and cut capped episode time from 948\,s to 576\,s.

\paragraph{Wrist singularity threshold ($0.21$\,rad vs.\ $0.35$\,rad).}
An aggressive post-contact wrist-tilt reset ($\theta_{\max}=0.21$\,rad) prematurely aborted valid pitched grasps on LIBERO-Pro ($49/80 \to 47/80$). Relaxing $\theta_{\max}$ to $0.35$\,rad intervened only on genuine cabinet-collision singularities, helping raise LIBERO-Pro to 55/80 (68.8\%).

\paragraph{Scoped loop-breakers and spatial serialization.}
Imposing a hard refusal after 15 consecutive read-only calls blocked legitimate multi-point \texttt{back\_project} sweeps on spatial tasks, while parallel tool batching (concurrency $P=8$) on duplicate-bowl scenes occasionally introduced state race conditions. Restricting hard caps solely to redundant \texttt{read\_task\_memory} ($\ge 2$) and static \texttt{read\_image} ($>6$) calls, paired with deterministic serial dispatch ($P=1$) on spatial disambiguation tasks, eliminated these failures while preserving $P=8$ concurrency elsewhere (reducing perception and VLA wall time by 16.9\%, from 30.2\,s under global $P=1$ serialization to 25.1\,s). 

\subsection{Horizon-Aware Clean-Scene Restart Budgeting}
\label{subsec:supp_restarts}

Under a fixed episode budget ($T_{\max}=1{,}800$\,s, $N_{\max}=100$ turns), clean-scene restarts recover rollouts where an early stochastic slip knocks an object out of reach. However, uniform reset partitioning introduces two failure modes across task horizons.

\paragraph{Turn-budget starvation under uniform splits.}
Under a uniform $3\times 36$-turn split, when Attempts~1 and~2 each consume their full 36-turn cap (72 turns total), Attempt~3 is left with only $100 - 72 = 28$ turns. Consequently, failed episodes terminate early at an average of 1{,}292\,s, leaving 508\,s of available wall-clock budget unused.

\paragraph{Horizon-aware budget allocation.}
Reallocating single-goal tasks to $2\times 820$\,s (50 turns per attempt) and multi-step long-horizon tasks (\texttt{libero\_10}) to a single $1\times 1{,}800$\,s (100-turn) budget eliminates turn starvation and prevents long-horizon episodes from aborting at 580\,s right after completing the first subgoal, lifting completion on LIBERO Standard ($67.5\% \to 80.0\%$) and LIBERO-Pro ($63.6\% \to 71.4\%$). Meanwhile, visual and camera perturbations in LIBERO-Plus still benefit from a third fresh scene reset ($3\times 560$\,s, 36 turns per attempt). Combining all three schedules---$3\times 560$\,s on LIBERO-Plus, $2\times 820$\,s on Standard and Pro single-goal tasks, and $1\times 1{,}800$\,s on long-horizon tasks---sustains 85.7\%--89.3\% success on LIBERO-Plus while maintaining 82.5\%--85.0\% on LIBERO Standard.

\begin{table}[t]
    \centering
    \caption{\textbf{Comparison of post-training strategies.}
    Results on the development gate (\texttt{seed=2}, up to 24 tasks)
    and the full contract (\texttt{seed=1}, 145 tasks).}
    \label{tab:supp_posttrain}
    \small
    \setlength{\tabcolsep}{3pt}
    \renewcommand{\arraystretch}{1.15}

    \begin{tabularx}{\textwidth}{@{}>{\raggedright\arraybackslash}p{0.18\textwidth} >{\raggedright\arraybackslash}X c c c c c@{}}
        \toprule
        \textbf{Method} & \textbf{Training Signal} & \multicolumn{3}{c}{\textbf{Development Gate}} & \multicolumn{2}{c}{\textbf{Full Contract}} \\
        \cmidrule(lr){3-5}\cmidrule(l){6-7}
        & & \textbf{SR (\%)} & \textbf{Std / Pro / Plus} & \textbf{Capped (s)} & \textbf{SR (\%)} & \textbf{Time (s)} \\
        \midrule
        Base SFT + MTP & Vision-frozen 64K SFT (\cref{eq:sft_loss}) & \textbf{87.5} (21/24) & \textbf{8/8}, 5/8, \textbf{8/8} & \textbf{498.7} & 72.4 (105/145) & 821.1 \\
        \addlinespace[2pt]
        Short-CoT Self-Distillation & Self-distill on $\leq 900$-token successful rollouts & 62.5 (15/24) & 7/8, 2/8, 6/8 & 836.0 & \multicolumn{2}{c}{\emph{Not evaluated}} \\
        Extended-CoT Self-Distillation & Self-distill on $\leq 1{,}800$-token successful rollouts & 50.0 (3/6) & --, 3/6, -- & 1064.6 & \multicolumn{2}{c}{\emph{Not evaluated}} \\
        \addlinespace[2pt]
        Online RLOO & Dual-clip PPO+TIS; 24 rollouts (70 turns) & 70.0 (14/20) & 4/7, 5/7, 5/6 & 730.9 & \multicolumn{2}{c}{\emph{Not evaluated}} \\
        Off-Policy CoT Distillation & 74\% teacher ($w_{\mathrm{think}}=0.2$) + 26\% student; $\mathrm{lr}=2\times10^{-5}$ & 66.7 (16/24) & 5/8, \textbf{7/8}, 4/8 & 842.3 & \textbf{77.9} (113/145) & 706.5 \\
        \textbf{Action-Only Distillation} & 50\% teacher ($w_{\mathrm{think}}=0$) + 50\% student; $\mathrm{lr}=8\times10^{-6}$ & \textbf{87.5} (21/24) & 7/8, 6/8, \textbf{8/8} & 563.7 & 75.9 (110/145) & \textbf{700.5} \\
        \bottomrule
    \end{tabularx}

    \vspace{3pt}
    \parbox{\textwidth}{\raggedright\scriptsize
    \emph{Note:} Methods rejected at the development gate were not evaluated on the full contract.
    Off-policy distillation uses routed inference; action-only distillation uses a single model.}
\end{table}

\subsection{Post-Training Explorations: Self-Distillation, Online RLOO, and Drift-Free Teacher Distillation}
\label{subsec:supp_posttrain}

We evaluate four post-training paradigms on top of the SFT Qwen3.5-9B backbone (\cref{tab:supp_posttrain}), trained strictly on held-out seeds (\texttt{inits 11--44}) with zero overlap with \texttt{seed=1} or \texttt{seed=2}.

\paragraph{Short-CoT self-distillation.}
To compress deliberation organically, we first fine-tuned LoRA adapters on the student's own fastest successful turns ($\le 900$ reasoning tokens in \texttt{lora-fast-v1}). While LIBERO Standard reached 7/8 on validation, LIBERO-Pro collapsed to 2/8 (25.0\%): filtering for short reasoning selectively discarded multi-object spatial disambiguation and taught premature grasping under object swaps. Widening the filter to $\le 1{,}800$ tokens (\texttt{lora-pro-v2}) still yielded only 3/6 on Pro because offline self-imitation cannot teach recovery behaviors absent from the student's repertoire.

\paragraph{Small-sample online RLOO.}
We next tested leave-one-out reinforcement learning (RLOO) with dual-clip PPO and truncated importance sampling (\texttt{rl-v007}) over live rollouts. Because each 50--100-turn closed-loop episode takes 5--15 minutes under 20\,Hz real-time physics, collecting 24 episodes yielded only 70 decision updates. Although \texttt{rl-v007} solved several hard goal-swap tasks, overall validation success dropped from 80.0\% (16/20) to 70.0\% (14/20), showing that pure on-policy policy gradients over sparse terminal rewards suffer from high variance under real-time simulation budgets.

\paragraph{Off-policy teacher distillation and CoT masking.}
Using DeepSeek-V4.1-Flash~\cite{deepseekv41flash} on non-evaluation seeds, we collected verified trajectories solving eight difficult tasks that had 0\% base-model success (including angled microwave mug insertion, dual moka-pot manipulation, and drawer-bowl disambiguation). Training a rank-32 LoRA (\texttt{rl-v008}, $\text{lr}=2\times 10^{-5}$, 74\% teacher / 26\% student turns) with weight $w_{\mathrm{think}}=0.20$ on teacher \texttt{<think>} tokens boosted Pro validation from 5/8 to 7/8 (87.5\%), confirming strong action transfer. However, Standard dropped from 8/8 to 5/8 and Plus from 8/8 to 4/8 because off-policy teacher chains-of-thought shifted Qwen's native deliberation style; routing \texttt{rl-v008} exclusively to Pro single-goal tasks achieved 77.9\% (113/145, 706.5\,s capped) on the full benchmark. In \texttt{rl-v009} (\cref{eq:post_loss,eq:token_weights}), we enforced a 50\%/50\% student--teacher turn balance across 212 solved episodes, lowered $\text{lr}$ to $8\times 10^{-6}$, and masked teacher \texttt{<think>} and \texttt{</think>} tokens completely ($w_{\mathrm{think}}=0.0$). This eliminated style drift, restoring validation success to 87.5\% (21/24) and achieving 75.9\% (110/145, 700.5\,s capped, 350.7\,s TTS) as a single unified checkpoint.

\paragraph{Time-aligned DAgger, specialist souping, and quantization.}
We further combined time-aligned DAgger with on-policy macro coalescing and concise-CoT refinement (\texttt{rl-v011b}, cutting per-turn deliberation tokens by 51\%), followed by Specialist Parameter Soup (\texttt{rl-soup-v3}). Served in \texttt{W8A16} with KL-aligned MTP drafting (259.8\,tok/s, 3.66 accepted tokens/step), this unified checkpoint lifted validation success to 95.8\% (23/24, 245.5\,s capped). On the full benchmark (\cref{tab:supp_progression}), it reached 62.8\%, 73.1\%, and 78.6\% completion at 200\,s, 400\,s, and 800\,s (116.6\,s mean TTS), and 83.4\% (121/145, 468.8\,s capped) with 3-stage clean-scene resets. Controlled quantization ablations on \texttt{seed=2} under identical scheduling further confirmed that near-lossless \texttt{W8A16} (91.7\%, 22/24) and hybrid \texttt{FP8}+\texttt{BF16} (79.2\%, 19/24) substantially outperform 4-bit \texttt{NVFP4} (62.5\%, 15/24), which suffers from 3D coordinate drift.
\begin{table}[t]
    \centering
    \small
    \caption{\textbf{End-to-end progression across contract evaluation panels (\texttt{seed=1}, $20$\,Hz $1\times$ clock, $n=145$).} Every row reports verified native simulator completion at 200\,s, 400\,s, 800\,s, and full $1{,}800$\,s budgets alongside conservation-checked timing.}
    \label{tab:supp_progression}
    \setlength{\tabcolsep}{3.5pt}
    \begin{tabularx}{\textwidth}{@{}l X c c c c c c@{}}
        \toprule
        \textbf{Panel} & \textbf{Key Architectural / Algorithmic Change} & \textbf{200\,s} & \textbf{400\,s} & \textbf{800\,s} & \textbf{1800\,s (Full)} & \textbf{Capped (s)} & \textbf{TTS / tok/s} \\
        \midrule
        \texttt{c2:dec} & Baseline Qwen3.5-9B SFT, no MTP ($n=71$) & --- & --- & --- & 53.5\% (38/71) & 1171.0 & 624.9\,s / 67.7 \\
        \texttt{c3} & + MTP-6 + $B_{\mathrm{think}}=2{,}048$ + \texttt{segment\_xyz}/\texttt{batch} & --- & --- & --- & 63.4\% (92/145) & 888.4 & 363.2\,s / 167.0 \\
        \texttt{c6} & + \texttt{mtp-v2} + KV block compaction + $3\times 580$\,s restarts & 31.7\% & 44.1\% & 57.9\% & 69.0\% (100/145) & 843.4 & 413.0\,s / 165.0 \\
        \texttt{c8} & + \texttt{opt8} ($0.35$\,rad un-wedge, horizon-aware restarts) & 29.0\% & 41.4\% & 55.2\% & 72.4\% (105/145) & 821.1 & 448.1\,s / 167.8 \\
        \texttt{c9} & + \texttt{opt9} ($0.0028$\,m grasp guard, crop scope, $P=8$, routed) & 37.2\% & 48.3\% & 64.8\% & 77.9\% (113/145) & 706.5 & 396.9\,s / 169.6 \\
        \texttt{c10} & + Unified \texttt{rl-v009} ($w_{\mathrm{think}}=0.0$) + denoised memory & 36.6\% & 49.7\% & 66.9\% & 75.9\% (110/145) & 700.5 & 350.7\,s / 168.6 \\
        \texttt{c13} & + On-policy KL-aligned MTP + \texttt{W8A16} serving & 51.0\% & 60.0\% & 71.0\% & 79.3\% (115/145) & 581.8 & 264.0\,s / 258.7 \\
        \texttt{c14} & + Time-aligned DAgger + Specialist Soup + 1-to-1 affinity & 57.2\% & 69.0\% & 80.0\% & 80.7\% (117/145) & 489.1 & 175.4\,s / 251.4 \\
        \texttt{c15} & + On-policy Macro \& Concise CoT only (w/o Soup) & 57.9\% & 67.6\% & 73.8\% & 73.8\% (107/145) & 565.1 & 126.6\,s / 250.9 \\
        \textbf{\texttt{c16}} & Macro + Concise CoT + Soup-v3 + aligned MTP (A800) & 62.8\% & 73.1\% & 78.6\% & 78.6\% (114/145) & 476.5 & \textbf{116.6\,s / 259.8} \\
        \texttt{c17} & + $R=3$ clean-scene perturbation resets (A800) & 53.8\% & 66.2\% & 80.7\% & 83.5\% (121/145) & 468.8 & 204.7\,s / 257.7 \\
        \textbf{\texttt{p5c8}} & \textbf{Ours: + multi-skill refinement \& zero-friction guards (PRO 5000)} & \textbf{67.6\%} & \textbf{74.5\%} & \textbf{85.5\%} & \textbf{89.7\% (130/145)} & \textbf{343.8} & 175.8\,s / 250.2 \\
        \bottomrule
    \end{tabularx}
\end{table}

\subsection{Full Progression Across Contract Panels (\texttt{c2}--\texttt{c17})}
\label{subsec:supp_progression}

\Cref{tab:supp_progression} summarizes the complete evolution across representative contract panels from \texttt{c2} through \texttt{c17}, raising full-contract completion from $53.5\%$ ($1{,}171.0$\,s) to \textbf{83.5\% (121/145, $468.8$\,s capped)} in \texttt{c17} and slashing mean time-to-success to \textbf{116.6\,s} ($62.8\%$/$73.1\%$/$78.6\%$ at 200/400/800\,s) in \texttt{c16}.

\subsection{Additional Fair Baseline Comparisons Across Frontier Models}
\label{subsec:supp_frontier_baselines}

\begin{table}[t]
\centering
\footnotesize
\setlength{\tabcolsep}{5.2pt}
\setlength{\aboverulesep}{0pt}
\setlength{\belowrulesep}{0pt}
\setlength{\extrarowheight}{0.8pt}
\renewcommand{\arraystretch}{1.05}
\caption{\textbf{System comparison using a shared GPT-6.2 Sol planner.} Success rates (\%) are reported within 200, 400, and 800\,s wall-clock budgets across LIBERO, LIBERO-Pro, and LIBERO-Plus. Each rate is computed over valid judged episodes for that method (coverage listed below). \textbf{Average} denotes the unweighted macro-average across the three benchmarks and is reported only for complete panels ($40/80/28$). Boldface indicates the highest observed rate in each column among methods sharing GPT-6.2 Sol; the final two rows report our native planner configurations for reference.}
\label{tab:supp_frontier_baselines}
\begin{adjustbox}{max width=\linewidth}
\begin{tabular}{@{}l !{\vrule width 0.6pt} ccc !{\vrule width 0.6pt} ccc !{\vrule width 0.6pt} ccc || ccc@{}}
\toprule
\multirow{2}{*}{\textbf{Method}}
& \multicolumn{3}{c!{\vrule width 0.6pt}}{\textbf{LIBERO (40)}}
& \multicolumn{3}{c!{\vrule width 0.6pt}}{\textbf{LIBERO-Pro (80)}}
& \multicolumn{3}{c||}{\textbf{LIBERO-Plus (28)}}
& \multicolumn{3}{c}{\textbf{Average}} \\
\cline{2-13}
 & 200\,s & 400\,s & 800\,s & 200\,s & 400\,s & 800\,s & 200\,s & 400\,s & 800\,s & 200\,s & 400\,s & 800\,s \\
\midrule
RPent~\cite{harness} & 2.5 & 15.0 & 37.5 & 5.0 & 21.3 & 55.0 & 0.0 & 10.7 & 53.6 & 2.5 & 15.7 & 48.7 \\
AgenticRoboRL~\cite{agenticroborl} & 2.9 & 5.9 & 26.5 & 0.0 & 1.3 & 25.0 & 0.0 & 3.6 & 50.0 & -- & -- & -- \\
CaP-Agent0~\cite{capx} & 2.5 & 2.5 & 30.0 & 0.0 & 2.5 & 33.8 & 0.0 & 7.7 & 46.2 & -- & -- & -- \\
RoboRSI~\cite{roborsi} & 0.0 & 2.5 & 10.0 & 0.0 & 0.0 & 6.3 & 0.0 & 0.0 & 3.7 & -- & -- & -- \\
VIA~\cite{via} & 0.0 & 17.5 & 35.0 & 1.3 & 13.8 & 35.0 & 0.0 & 14.3 & 57.1 & 0.4 & 15.2 & 42.4 \\
\midrule
\rowcolor{blue!8}
\textbf{RA-RT (GPT-6.2 Sol)} & \textbf{5.0} & \textbf{50.0} & \textbf{80.0} & \textbf{13.8} & \textbf{76.3} & \textbf{86.3} & \textbf{28.6} & \textbf{78.6} & \textbf{82.1} & \textbf{15.8} & \textbf{68.3} & \textbf{82.8} \\
\midrule
\rowcolor{purple!6}
\textbf{RA-RT (DeepSeek)} & 95.0 & 100.0 & 100.0 & 62.5 & 76.3 & 80.0 & 82.1 & 96.4 & 100.0 & 79.9 & 90.9 & 93.3 \\
\rowcolor{orange!10}
\textbf{RA-RT (Qwen3.5-9B)} & 90.0 & 92.5 & 97.5 & 48.8 & 57.5 & 72.5 & 82.1 & 89.3 & 96.4 & 73.6 & 79.8 & 88.8 \\
\bottomrule
\end{tabular}
\end{adjustbox}

\vspace{3pt}
\begin{minipage}{\linewidth}
\scriptsize
\textit{Judged coverage (LIBERO / Pro / Plus):} RPent, VIA, and RA-RT (GPT-6.2 Sol) 40/80/28; AgenticRoboRL 34/80/28; CaP-Agent0 40/80/13; RoboRSI 40/80/27.
\end{minipage}
\end{table}
In the main paper (\cref{tab:benchmark_results}), all API-backed baselines (RPent~\cite{harness}, CaP-Agent0~\cite{capx}, ASPIRE~\cite{aspire}, RoboRSI~\cite{roborsi}, and VIA~\cite{via}) are evaluated under a unified DeepSeek-V4.1-Flash~\cite{deepseekv41flash} backbone, while AgenticRoboRL~\cite{agenticroborl} is evaluated using its native local Qwen3.5-9B models. Correspondingly, our framework is evaluated under both configurations (DeepSeek-V4.1-Flash and our Qwen3.5-9B student). This ensures that architectural differences in skill scheduling and visual grounding are isolated from VLM backbone disparities.

To definitively demonstrate that our performance advantages generalize across different frontier models and are not overfitted to a specific API, we re-evaluated both our agent and \textbf{all applicable baselines---including AgenticRoboRL}---using GPT-6.2-Sol as the underlying visual-language backbone. 

As shown in \cref{tab:supp_frontier_baselines}, all methods were subjected to the exact same $1\times$ 20\,Hz real-time simulation protocol (1800\,s wall-clock budget). The results confirm that substituting the backbone with GPT-6.2-Sol yields consistent relative performance trends. Even with a different frontier model powering the reasoning, \textbf{Ours (GPT-6.2-Sol)} significantly outperforms all GPT-6.2-Sol-powered baselines. Furthermore, compared to our main reference configurations (DeepSeek and Qwen3.5-9B), our framework demonstrates robust cross-model generalizability, proving that its superiority stems fundamentally from efficient asynchronous scheduling and robust guardrails.

\begin{table}[t]
  \centering
  \caption{Planner-callable skills in the RPent LIBERO adapter.}
  \label{tab:supp_libero_skills}
  \small
  \setlength{\tabcolsep}{4pt}
  \renewcommand{\arraystretch}{1.08}
  \begin{tabularx}{\columnwidth}{@{}l>{\raggedright\arraybackslash}X@{}}
    \toprule
    \textbf{Skill} & \textbf{Function} \\
    \midrule
    \multicolumn{2}{@{}l}{\textit{Learned manipulation}} \\
    \texttt{pi0\_pick}    & Execute a language-conditioned grasp in closed loop. \\
    \texttt{pi0\_doubled} & Execute a contact action, such as turning a knob. \\
    \addlinespace
    \multicolumn{2}{@{}l}{\textit{Scripted motion and gripper control}} \\
    \texttt{move\_to}      & Move the end effector to a world-frame position. \\
    \texttt{move\_pose}    & Jointly control position, pitch, and yaw. \\
    \texttt{rotate\_wrist} & Adjust wrist yaw at fixed end-effector position. \\
    \texttt{rotate\_pitch} & Adjust wrist pitch at fixed end-effector position. \\
    \texttt{set\_gripper}  & Actuate the gripper while holding the arm pose. \\
    \texttt{release}       & Open the gripper. \\
    \addlinespace
    \multicolumn{2}{@{}l}{\textit{Observation and geometry}} \\
    \texttt{view\_env\_state}   & Retrieve recorded state and camera images. \\
    \texttt{view\_camera\_meta} & Retrieve camera metadata for a recorded step. \\
    \texttt{segment}           & Use SAM~3~\cite{sam3} and registered depth to estimate
                                 3D geometry from a text- or point-prompted mask. \\
    \texttt{back\_project}     & Map an image pixel to world coordinates. \\
    \texttt{plan\_placement}   & Estimate placement alignment and footprint fit
                                 from the held-object and destination masks. \\
    \bottomrule
  \end{tabularx}
\end{table}

\subsection{Simulation Skill Library}
\label{subsec:supp_real_skill_library}

We use the RPent skill library~\cite{harness} across LIBERO,
LIBERO-Pro, and LIBERO-Plus. The two learned skills in
Table~\ref{tab:supp_libero_skills} share a frozen LIBERO-tuned
$\pi_{0.5}$ policy~\cite{pi05,pi0}.

\subsection{Simulation Results on RoboCasa and RoboTwin}
\label{subsec:supp_robocasa_robotwin}

To evaluate generalization beyond LIBERO tabletop suites, we compare official RPent~\cite{harness} against \textbf{RA-RT} on RoboCasa365 Target50~\cite{robocasa} and RoboTwin C2R~\cite{robotwin}. For each benchmark, we evaluate a fixed panel of 100 task--initialization pairs split evenly between atomic (50) and composite (50) tasks. On RoboCasa, the 50 composite tasks follow the benchmark's native split of 25 seen and 25 unseen configurations, with wall-clock budgets of $1{,}800$\,s for atomic tasks and $3{,}600$\,s for composite tasks. On RoboTwin, all 100 episodes use the \texttt{demo\_randomized} setting with a $4{,}800$\,s budget. Both methods use GPT-6.2-Sol at medium reasoning effort, share identical low-level controllers, tasks, random seeds, and language instructions within each benchmark, and retain their respective native memory configurations.

\begin{table}[t]
\centering
\caption{\textbf{Fine-grained comparison on RoboCasa365 Target50 and RoboTwin C2R using GPT-6.2-Sol.} \textbf{Solved} reports completions over judged episodes under full native budgets ($1{,}800$\,s RoboCasa atomic, $3{,}600$\,s RoboCasa composite, and $4{,}800$\,s RoboTwin). Intermediate columns report cumulative success rates (\%) from $400$\,s to $1{,}800$\,s, and \textbf{TTS} denotes mean time-to-success on solved episodes. Dashes mark unreported RA-RT results for the atomic and composite RoboTwin splits.}
\label{tab:supp_robocasa_robotwin}
\resizebox{\linewidth}{!}{
\setlength{\tabcolsep}{3.6pt}
\setlength{\aboverulesep}{0pt}
\setlength{\belowrulesep}{0pt}
\setlength{\extrarowheight}{0.8pt}
\renewcommand{\arraystretch}{1.05}
\begin{tabular}{@{}ll !{\vrule width 0.6pt} c !{\vrule width 0.6pt} ccccc !{\vrule width 0.6pt} c@{}}
\toprule
\textbf{Benchmark / Split} & \textbf{Method} & \textbf{Solved} & \textbf{400\,s} & \textbf{600\,s} & \textbf{800\,s} & \textbf{1200\,s} & \textbf{1800\,s} & \textbf{TTS (s)} \\
\midrule
\multirow{2}{*}{RoboCasa Atomic}
 & RPent & 38/50 & 66.0 & 68.0 & 68.0 & 72.0 & 76.0 & 206 \\
 & \cellcolor{purple!8}\textbf{RA-RT} & \cellcolor{purple!8}\textbf{40/50} & \cellcolor{purple!8}\textbf{74.0} & \cellcolor{purple!8}\textbf{80.0} & \cellcolor{purple!8}\textbf{80.0} & \cellcolor{purple!8}\textbf{80.0} & \cellcolor{purple!8}\textbf{80.0} & \cellcolor{purple!8}\textbf{132} \\
\midrule
\multirow{2}{*}{RoboCasa Composite}
 & RPent & 12/50 & 10.0 & 12.0 & 14.0 & 20.0 & 22.0 & 708 \\
 & \cellcolor{purple!8}\textbf{RA-RT} & \cellcolor{purple!8}\textbf{19/39} & \cellcolor{purple!8}\textbf{30.8} & \cellcolor{purple!8}\textbf{38.5} & \cellcolor{purple!8}\textbf{48.7} & \cellcolor{purple!8}\textbf{48.7} & \cellcolor{purple!8}\textbf{48.7} & \cellcolor{purple!8}\textbf{372} \\
\midrule
\multirow{2}{*}{RoboTwin Atomic}
 & RPent & 38/50 & 68.0 & 72.0 & 74.0 & 76.0 & 76.0 & 189 \\
 & \cellcolor{purple!8}\textbf{RA-RT} & \cellcolor{purple!8}\textemdash & \cellcolor{purple!8}\textemdash & \cellcolor{purple!8}\textemdash & \cellcolor{purple!8}\textemdash & \cellcolor{purple!8}\textemdash & \cellcolor{purple!8}\textemdash & \cellcolor{purple!8}\textemdash \\
\midrule
\multirow{2}{*}{RoboTwin Composite}
 & RPent & 28/50 & 40.0 & 50.0 & 52.0 & 52.0 & 56.0 & 358 \\
 & \cellcolor{purple!8}\textbf{RA-RT} & \cellcolor{purple!8}\textemdash & \cellcolor{purple!8}\textemdash & \cellcolor{purple!8}\textemdash & \cellcolor{purple!8}\textemdash & \cellcolor{purple!8}\textemdash & \cellcolor{purple!8}\textemdash & \cellcolor{purple!8}\textemdash \\
\bottomrule
\end{tabular}
}
\end{table}

As shown in \cref{tab:supp_robocasa_robotwin}, \textbf{RA-RT} consistently improves both completion rate and execution speed over official RPent across RoboCasa task horizons. On single-stage atomic tasks, RA-RT raises completion from 76.0\% (38/50) to \textbf{80.0\%} (40/50), reaches its full 80.0\% ceiling within $600$\,s, and cuts mean time-to-success by \textbf{35.9\%} (from $206$\,s to \textbf{$132$\,s}). The advantage widens substantially on multi-stage composite kitchen tasks, where serial execution in RPent frequently stalls during articulated fixture manipulation and error recovery: RA-RT more than doubles the $1{,}800$\,s success rate from 22.0\% to \textbf{48.7\%} (19/39 vs.\ 12/50 under the full $3{,}600$\,s budget), solves all 19 completed episodes within $800$\,s, and reduces mean TTS by \textbf{47.5\%} (from $708$\,s to \textbf{$372$\,s}). On RoboTwin, official RPent reaches 76.0\% (38/50, $189$\,s TTS) on atomic tasks and 56.0\% (28/50, $358$\,s TTS) on composite tasks.

\subsection{Full-1800\,s Vanilla Serial Baseline and Zero-Memory Comparison}
\label{subsec:supp_vanilla_serial}

\begin{figure}[t]
    \centering
    \includegraphics[width=\textwidth]{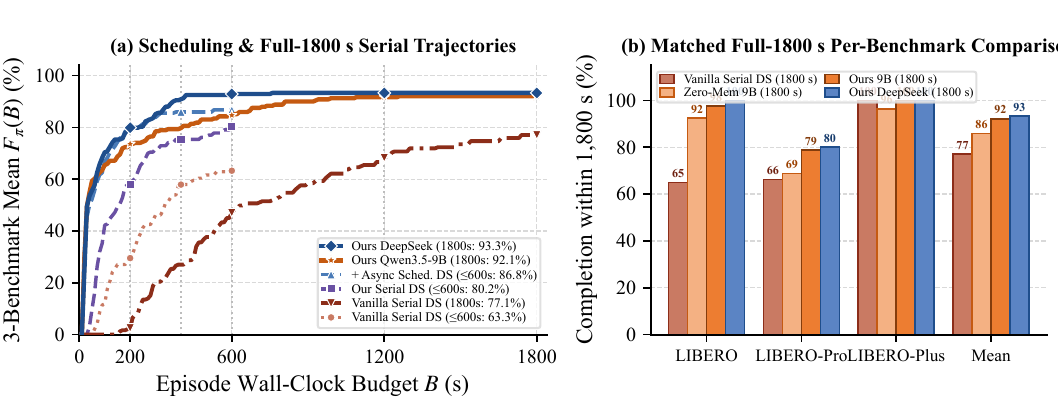}
    \caption{\textbf{Controlled scheduling trajectories and matched $1{,}800$\,s per-benchmark comparison ($20$\,Hz real-time pacing).} \textbf{(a)} Three-benchmark mean completion $F_{\pi}(B)$ over $B \in [0, 1{,}800]$\,s comparing vanilla upstream serial execution (\texttt{f70d720}, both $\le 600$\,s low-concurrency and full $1{,}800$\,s runs), our safeguard-matched serial and asynchronous DeepSeek ablations ($\le 600$\,s, zero notes), and full RA-RT (DeepSeek / Qwen3.5-9B). \textbf{(b)} Completion within the full $1{,}800$\,s budget across LIBERO, LIBERO-Pro, LIBERO-Plus, and their unweighted mean, including our pure cold-start zero-memory 9B planner.}
    \label{fig:supp_ablation_dss0}
\end{figure}

To remove the $600$\,s horizon truncation of our initial serial check (\texttt{dss0}, $59.3\%$ task rate), we evaluated unmodified upstream RPent (commit \texttt{f70d720}, official DeepSeek-V4.1-Flash API) up to the full $B = 1{,}800$\,s budget ($N_{\max} = 360$ turns; \texttt{dss1800}, \cref{fig:supp_ablation_dss0}) under pure single-step serial execution, cold zero-memory, and $20$\,Hz pacing. All $38$ unsolved episodes ran to the full $1{,}800$\,s ceiling without premature termination. Relaxing the cap from $600$\,s to $1{,}800$\,s lifts vanilla serial DeepSeek by $+21$ tasks to $107/145$ ($73.8\%$ overall, $77.1\%$ three-benchmark mean, $917.7$\,s capped time): while simpler perturbations saturate (e.g., $100.0\%$ on LIBERO-Plus and $10/10$ on \texttt{object\_swap/task}), long-horizon composition remains bottlenecked ($1/9$ on \texttt{libero\_10\_task}). Across matched $1{,}800$\,s evaluations on all $145$ tasks, performance scales monotonically from vanilla serial 9B ($22.1\%$, $1{,}551.7$\,s capped) and full-$1{,}800$\,s serial DeepSeek ($73.8\%$, $917.7$\,s capped) to our cold-start zero-memory 9B planner on RTX PRO 5000 ($82.1\%$, $85.9\%$ mean, $435.1$\,s capped)---achieving $+8.8$\,pp higher benchmark mean at $2.11\times$ faster speed under identical zero-memory rules---and finally to complete RA-RT 9B ($88.3\%$--$89.7\%$, $343.8$--$387.1$\,s capped, with $100.0\%$ in $39.9$\,s mean time on LIBERO Standard).

\subsection{Zero-Leakage Generalization on Unseen Dual-Platform MuJoCo Tasks}
\label{subsec:supp_mujoco_unseen50}

To test cross-embodiment generalization under strict zero simulation-target leakage, we sealed an unseen $50$-task dual-platform MuJoCo benchmark ($25$ RealMan single-/dual-arm tasks and $25$ ReBot/B601 wrist-camera tasks; zero trajectories or images from the $500$-task environment pool used in training). While a LIBERO-specialized checkpoint suffers tool-schema hallucination ($10.0\%$), pairing Qwen3.5-9B with our unified hardware-safe skill contract lifts zero-shot accuracy from $28.0\%$ ($14/50$) to $66.0\%$ ($33/50$), and merging LoRA adapters trained purely on disjoint cross-embodiment anchors reaches $70.0\%$ ($35/50$, zero runtime errors; $56.0\%$ [$14/25$] on RealMan, matching the official DeepSeek API reference on the same ledger, and $84.0\%$ [$21/25$] on ReBot), with the zero-leakage 9B family union reaching $82.0\%$ ($41/50$).
